# Supplementary material for: When to Boost: How Dose Timing Determines the Epidemic Threshold
Source: arXiv:2502.16715 ancillary file (2025-02-23)
Supplement: Supplementary file 1 [file SM_whenToBoost.pdf]

## Supplemental Material

Alessandro Celestini,<sup>1</sup> Francesca Colaiori,<sup>2,3</sup> Stefano Guarino,<sup>1</sup> Enrico Mastrostefano,<sup>1</sup> Francesca Pelusi,<sup>4</sup> and Lena Rebecca Zastrow<sup>5</sup>

<sup>1</sup>*CNR, Institute for Applied Mathematics, Rome, Italy*

<sup>2</sup>*CNR, Institute for Complex Systems, Rome, Italy*

<sup>3</sup>*Department of Physics, Sapienza University, Rome, Italy*

<sup>4</sup>*CNR, Institute for Applied Mathematics, Naples, Italy*

<sup>5</sup>*ISPRA, Department of the Geological Survey of Italy, Rome, Italy*

(Dated: February 23, 2025)

### NATURE OF THE TRANSITION AND STABILITY OF THE ENDEMIC SOLUTION

We demonstrate that the transition from the absorbing, inactive phase with  $\rho = 0$  to the stationary endemic phase with  $\rho > 0$  is continuous. We recall here the set of differential equations describing the dynamics of the  $S^3I^2$  model:

$$\begin{cases} \dot{s}_0 = -\lambda \rho s_0 - c\alpha s_0 + \eta_1 s_1 + \eta_2 s_2 \\ \dot{s}_1 = -\sigma_1 \lambda \rho s_1 + c\alpha s_0 - c(1-\alpha)s_1 - \eta_1 s_1 + \gamma \rho_1 \\ \dot{s}_2 = -\sigma_2 \lambda \rho s_2 + c(1-\alpha)s_1 - \eta_2 s_2 + \gamma \rho_2 \\ \dot{\rho}_1 = \lambda \rho s_0 - \gamma \rho_1 \\ \dot{\rho}_2 = \lambda \rho (\sigma_1 s_1 + \sigma_2 s_2) - \gamma \rho_2 \end{cases} \quad (1)$$

where,  $s_i$  and  $\rho_i$  indicate the population fraction in the three susceptible and two infected states,  $\lambda$  is the transmission rate, and  $s_1 + s_2 + s_3 + \rho_1 + \rho_2 = 1$ . The dependency on time is understood. The parameters in Eq. 1 satisfy:  $0 \leq \sigma_2 \leq \sigma_1 \leq 1$ ,  $0 \leq \eta_2 \leq \eta_1$ ,  $0 \leq \alpha \leq 1$ . At stationarity, the total fraction of infected  $\rho = \rho_1 + \rho_2$  is constant; thus we get

$$\rho (\lambda (s_0 + \sigma_1 s_1 + \sigma_2 s_2) - \gamma) = 0. \quad (2)$$

This equation is always satisfied in the inactive phase with  $\rho = 0$ , while, in the endemic phase, corresponding to a solution with  $\rho \neq 0$ , it requires

$$s_0 + \sigma_1 s_1 + \sigma_2 s_2 = \gamma / \lambda. \quad (3)$$

The endemic phase can thus be defined in terms of the four variables  $s_0, s_1, s_2, \rho$  by

$$\begin{cases} X_0(\rho) s_0 = (\eta_1 + X_1(\rho)) s_1 \\ \eta_2 s_2 = X_1(\rho) s_1 \\ s_0 + \sigma_1 s_1 + \sigma_2 s_2 - \gamma / \lambda = 0 \\ \rho + s_0 + s_1 + s_2 - 1 = 0 \end{cases} \quad (4)$$

where  $X_0(\rho) = \lambda \rho + c\alpha$ , and  $X_1(\rho) = \sigma_1 \lambda \rho + c(1-\alpha)$ . By eliminating  $s_0$  we obtain

$$\begin{cases} \eta_2 s_2 = X_1(\rho) s_1 \\ ((\eta_1 + X_1(\rho)) / X_0(\rho) + \sigma_1 + \sigma_2 X_1(\rho) / \eta_2) s_1 = \gamma / \lambda \\ \rho + (1 - \sigma_1) s_1 + (1 - \sigma_2) s_2 - 1 + \gamma / \lambda = 0, \end{cases} \quad (5)$$

which gives the following self-consistent equation for  $\rho$

$$\rho = g(\rho) \quad (6)$$

with

$$g(\rho) = 1 - \frac{\gamma}{\lambda} - \frac{\gamma}{\lambda} \frac{\eta_2 (1 - \sigma_1) X_0(\rho) + (1 - \sigma_2) X_0(\rho) X_1(\rho)}{\eta_2 (\eta_1 + X_1(\rho)) + \eta_2 \sigma_1 X_0(\rho) + \sigma_2 X_0(\rho) X_1(\rho)}. \quad (7)$$

After a little algebra, it is easy to show that  $g'(\rho) \leq 0$  for all combinations of parameters within the allowed ranges. Moreover,  $g(0) < 1$  for any finite value of  $\lambda$ . As expected,  $g(\rho) = 1 - \gamma / \lambda$  for  $\sigma_1 = \sigma_2 = 1$ , when the  $S^3I^2$  model

reduces to the standard SIS model, and  $\lambda_c/\gamma = 1$ . The condition for Eq. (6) to have a solution with  $\rho > 0$  is therefore that  $g(0) > 0$ , which, in turn, implies  $\lambda > \lambda_c$  with

$$\lambda_c = \gamma \frac{\eta_2(\eta_1 + c) + c^2\alpha(1 - \alpha)}{\eta_2(\eta_1 + c) - \eta_2c(1 - \sigma_1) + \sigma_2c^2\alpha(1 - \alpha)}. \quad (8)$$

The transition is therefore continuous, and the  $\lambda_c$  coincides with the value where the inactive phase becomes unstable (cfr. Eq. 4 in the main paper).

## NETWORKS USED FOR THE NUMERICAL SIMULATIONS

We performed quasistationary (QS) numerical simulations of the  $S^3I^2$  model on three different networks: i) an Erdős–Rényi–Gilbert (ER) graph [1] ii) the Enron email network [2, 3], and iii) a geometric random graph generated using the  $S^1$  model[4]. The structural properties of the networks used are summarized in Table I.

|       | $N$   | $\langle k \rangle$ | $T$     | $C$    | $r$     |
|-------|-------|---------------------|---------|--------|---------|
| ER    | 50000 | 10.84               | 0.00024 | 0.0002 | 0.00037 |
| Enron | 36692 | 10.02               | 0.08531 | 0.4970 | -0.11   |
| $S^1$ | 50000 | 10.32               | 0.04619 | 0.4757 | -0.051  |

TABLE I. Structural properties of the networks used in the simulations: number of nodes ( $N$ ), average degree ( $\langle k \rangle$ ), transitivity ( $T$ ), average clustering coefficient ( $C$ ), and assortativity ( $r$ ).

The numerical analysis of SIS-type dynamics in finite-size systems is challenging, since for sufficiently long times an absorbing state is always visited, implying that the system ends being trapped in the absorbing-state, the unique real stationary state. An alternative is to consider the so-called quasistationary state where the original dynamics is perturbed to skip the absorbing state and several methods have been proposed to sample quasistationary regime [5, 6]. We used the *reactivation per activity time* (RAT) method, proposed by Costa and Ferreira [6]. The RAT method consists of reactivating a random selection of nodes, after the dynamics has fallen into an absorbing state. The activation of each node is based on its history of activity, nodes that were active for longer periods of time are more likely to be reactivated. The reactivation is performed as an independent Bernoulli process where the activation probability of each node is proportional to the activity time of the node. We simulated the  $S^3I^2$  model using EoN (Epidemics on Networks) [7, 8], a Python module designed to study infectious processes spreading in networks. Specifically, we used the Gillespie implementation provided by EoN and the NetworkX package [9] to implement the  $S^3I^2$  model. The model is implemented as a directed NetworkX graph, and is passed as argument to the Gillespie algorithm. We considered an initial condition in which all nodes are infected and we studied the QS density  $\langle \rho \rangle$  of infectious population versus the individual transmission rate  $\beta$ , for different values of the priority index  $\alpha$ , averages were computed over 50 realizations. Simulations are divided into two phases, a relaxation phase and an averaging phase. The QS distribution  $P_{qs}(v)$  is computed during the averaging phase, where  $P_{qs}(v)$  is the probability that  $v$  elements are active in the QS regime.  $P_{qs}(v)$  is used to compute  $\langle \rho \rangle$  and  $\langle \rho^2 \rangle$  the two quantities needed to compute the variability  $\Delta$ . We used the variability measure, whose usage has been proposed in [10], to estimate the critical individual transmission rate  $\beta_c$ .

- 
- [1] E. N. Gilbert, The Annals of Mathematical Statistics **30**, 1141 (1959), 2237458.
  - [2] J. Leskovec and A. Krevl, SNAP Datasets: Stanford large network dataset collection, <http://snap.stanford.edu/data> (2014).
  - [3] B. Klimt and Y. Yang, in *CEAS*, Vol. 4 (2004) p. 1.
  - [4] M. Á. Serrano, D. Krioukov, and M. Boguná, Physical Review Letters **100**, 078701 (2008).
  - [5] R. S. Sander, G. S. Costa, and S. C. Ferreira, Physical Review E **94**, 042308 (2016).
  - [6] G. S. Costa and S. C. Ferreira, Computer Physics Communications **267**, 108046 (2021).
  - [7] I. Z. Kiss, J. C. Miller, P. L. Simon, *et al.*, Cham: Springer **598**, 31 (2017).
  - [8] J. C. Miller and T. Ting, Journal of Open Source Software **4**, 1731 (2019).
  - [9] <https://networkx.org>.
  - [10] P. Shu, W. Wang, M. Tang, and Y. Do, Chaos: An Interdisciplinary Journal of Nonlinear Science **25** (2015).
